# Supplementary material for: Fragment size density estimator for shrinkage-induced fracture based on a physics-informed neural network
Source: arXiv:2507.11799 ancillary file (2025-08-13)
Supplement: Supplementary file 1 [file supplemental.pdf]

# Supplemental Materials: Fragment Size Density Estimator for Shrinkage-Induced Fracture Based on Physics-Informed Neural Network

Shin-ichi Ito[1] *

[1]*Earthquake Research Institute, The University of Tokyo, 1-1-1 Yayoi, Bunkyo-ku, Tokyo, Japan, 113-0032*

## 1. Architecture dependency

In this section, we assess how two key architectural hyper-parameters—network width and depth—influence predictive accuracy and training time. We vary both the number of skip-connected layers and their widths, while holding all other settings identical to those in the main text. The experiments examine layer widths of 64 and 128 units and depths of 1, 3, and 6 layers. For each configuration, we perform ten independent runs with distinct random initializations and optimize using the strategy (iv) described in Section 4.2. The total number of trainable parameters for each architecture is listed in Table I.

Figure 1 presents the final training loss achieved by each architecture versus its corresponding training time. In every case, both the final training loss and the time required to reach it are highly sensitive to the random seed. Within the range explored, the architecture with width = 128 and the number of skip-connected layers = 1 delivers the lowest average training loss, with the best run reaching approximately $10^{-10}$. Although a larger parameter count is often presumed to confer greater representational power, these results underscore that the potential is not automatically realized. Figures 2 and 3 plot the final test losses, $L_{2,1}^{\text{test}}$ and $L_{2,2}^{\text{test}}$, respectively, against training time. The trends mirror those observed for the training loss: architectures that attain lower training losses consistently exhibit lower test losses. Within the range of random initializations investigated, no evidence of overtraining is observed.

*ito@eri.u-tokyo.ac.jp

## 2. Levenberg–Marquardt optimization

In this section, we recast the loss function (Eq. (13)) into a sum-of-squared-residuals (SSR) form to apply the Levenberg–Marquardt algorithm introduced by Jnini and Vella.[1)]

Let $\Psi$ denote the concatenated vector of neural-network parameters $\theta$ and $\phi$, introduced for notational convenience. Following the discretization scheme outlined in Section 4.1, we represent the quadrature nodes for the integral in Eq. (9) by $x_k$ $(k = 1, \ldots, n_x)$ and their associated weights by $\Delta x_k$. Likewise, the two-dimensional parameter domain of $\alpha$ and $\gamma$ is discretized into nodes $\alpha_i$ $(i = 1, \ldots, n_\alpha)$ and $\gamma_j$ $(j = 1, \ldots, n_\gamma)$, with composite weights $s_{i,j}$ that encode the assumed log-uniform distributions of $\alpha$ and $\gamma$. With this discretization, the loss function can be written explicitly as

$$\begin{aligned} L(\Psi) = &\frac{1}{2} \sum_{i=1}^{n_\alpha} \sum_{j=1}^{n_\gamma} \sum_{k=1}^{n_x} s_{i,j} \Delta x_k g(x_k) \left( I \left[ x_k, p_\theta(x_k; \alpha_i, \gamma_j), a_\phi(\alpha_i, \gamma_j), \alpha_i, \gamma_j \right] \right)^2 \\ &+ \frac{1}{2} w_2 \sum_{i=1}^{n_\alpha} \sum_{j=1}^{n_\gamma} s_{i,j} \left[ 1 - \int_0^\infty dx\, p_\theta(x; \alpha_i, \gamma_j) \right]^2 \\ &+ \frac{1}{2} w_3 \sum_{i=1}^{n_\alpha} \sum_{j=1}^{n_\gamma} s_{i,j} \left[ 1 - \int_0^\infty dx\, x p_\theta(x; \alpha_i, \gamma_j) \right]^2 , \end{aligned} \tag{S.1}$$

where, in this explanation, the integrals in the second and third terms are left in continuous form, because their discretization is immaterial to the SSR construction and is therefore omitted to avoid unnecessary complexity. In actual computation, these integrals and that involved in $I$ are discretized following the discretization manner shown in Section. 4.1. The discretized loss (Eq. (S.1)) can be written as a sum of $M = n_\alpha n_\gamma (n_x + 2)$ squared residuals

$$L(\Psi) = \frac{1}{2} \sum_{m=1}^{M} r_m^2 = \frac{1}{2} \mathbf{r}^\top \mathbf{r}, \tag{S.2}$$

where

$$\begin{aligned} r_{i+(j-1)n_\alpha+(k-1)n_\alpha n_\gamma}(\Psi) &= \sqrt{s_{i,j} \Delta x_k g(x_k)} I \left[ x_k, p_\theta(x_k; \alpha_i, \gamma_j), a_\phi(\alpha_i, \gamma_j), \alpha_i, \gamma_j \right] \\ &\qquad \left( 1 \le i \le n_\alpha, 1 \le j \le n_\gamma, 1 \le k \le n_x \right), \\ r_{i+(j-1)n_\alpha+n_x n_\alpha n_\gamma}(\Psi) &= \sqrt{s_{i,j} w_2} \left[ 1 - \int_0^\infty dx\, p_\theta(x; \alpha_i, \gamma_j) \right] \quad \left( 1 \le i \le n_\alpha, 1 \le j \le n_\gamma \right), \\ r_{i+(j-1)n_\alpha+(n_x+1)n_\alpha n_\gamma}(\Psi) &= \sqrt{s_{i,j} w_3} \left[ 1 - \int_0^\infty dx\, x p_\theta(x; \alpha_i, \gamma_j) \right] \quad \left( 1 \le i \le n_\alpha, 1 \le j \le n_\gamma \right). \end{aligned} \tag{S.3}$$

In the main text, we have chosen $n_\alpha = 16$, $n_\gamma = 16$, and $n_x = 64$, which gives a total of $M = 16,896$ residuals.

Let $N$ denote the dimension of $\Psi$ (i.e., the total number of trainable parameters). To minimize the SSR objective in Eq. (S.2), the Levenberg–Marquardt (LM) algorithm—a damped Gauss–Newton algorithm—determines the descent direction $\mathbf{d} \in \mathbb{R}^N$ by solving

$$(\mathbf{J}^\top \mathbf{J} + \lambda \mathbf{I}_N)\,\mathbf{d} = -\mathbf{J}^\top \mathbf{r} \;(= -\nabla_\Psi L), \tag{S.4}$$

where $\mathbf{I}_N$ is the $N \times N$ identity matrix, $\lambda > 0$ is an adaptively chosen damping parameter, and the Jacobian

$$\mathbf{J} = \frac{\partial \mathbf{r}}{\partial \Psi}. \tag{S.5}$$

collects the first derivatives of the residual vector $\mathbf{r}$. In ordinary neural-network tasks, $N$ is extremely large, so solving the linear system demands both $O(N^2)$ memory and $O(N^3)$ floating-point operations, rendering a direct solution impractical. Recently, Jnini and Vella[1) have proposed a reformulation technique that reduces this cost by working in residual space rather than parameter space. Introducing an auxiliary vector $\mathbf{y} \in \mathbb{R}^M$, their reformulation is given by

$$(\mathbf{J}\mathbf{J}^\top + \lambda \mathbf{I}_M)\,\mathbf{y} = -\mathbf{J}\nabla_\Psi L, \tag{S.6}$$

$$\mathbf{d} = -\frac{1}{\lambda}\left(\mathbf{J}^\top \mathbf{y} + \nabla_\Psi L\right). \tag{S.7}$$

Its equivalence to the standard LM update (Eq. (S.4)) is immediate:

$$\begin{aligned}
(\mathbf{J}^\top \mathbf{J} + \lambda \mathbf{I}_N)\,\mathbf{d} &= -\frac{1}{\lambda}(\mathbf{J}^\top \mathbf{J} + \lambda \mathbf{I}_N)(\mathbf{J}^\top \mathbf{y} + \nabla_\Psi L) \qquad \text{(Substituting Eq. (S.7))}\\
&= -\frac{1}{\lambda}(\mathbf{J}^\top \mathbf{J} + \lambda \mathbf{I}_N)\,\mathbf{J}^\top \mathbf{y} - \frac{1}{\lambda}(\mathbf{J}^\top \mathbf{J} + \lambda \mathbf{I}_N)\,\nabla_\Psi L\\
&= -\frac{1}{\lambda}\mathbf{J}^\top(\mathbf{J}\mathbf{J}^\top + \lambda \mathbf{I}_M)\,\mathbf{y} - \frac{1}{\lambda}(\mathbf{J}^\top \mathbf{J} + \lambda \mathbf{I}_N)\,\nabla_\Psi L\\
&= \frac{1}{\lambda}\mathbf{J}^\top \mathbf{J}\nabla_\Psi L - \frac{1}{\lambda}(\mathbf{J}^\top \mathbf{J} + \lambda \mathbf{I}_N)\,\nabla_\Psi L \qquad \text{(Substituting Eq. (S.6))}\\
&= -\nabla_\Psi L.
\end{aligned} \tag{S.8}$$

Solving Eqs. (S.6) and (S.7) requires $O(MN)$ memory—to store the $M \times N$ Jacobian—and $O(M^3)$ floating-point operations for the linear solve. When $M \ll N$, which is typical for PINN problems, this reformulation yields a marked reduction in both storage and computational cost compared with the $O(N^2)$ memory and $O(N^3)$ work demanded by the standard LM scheme.

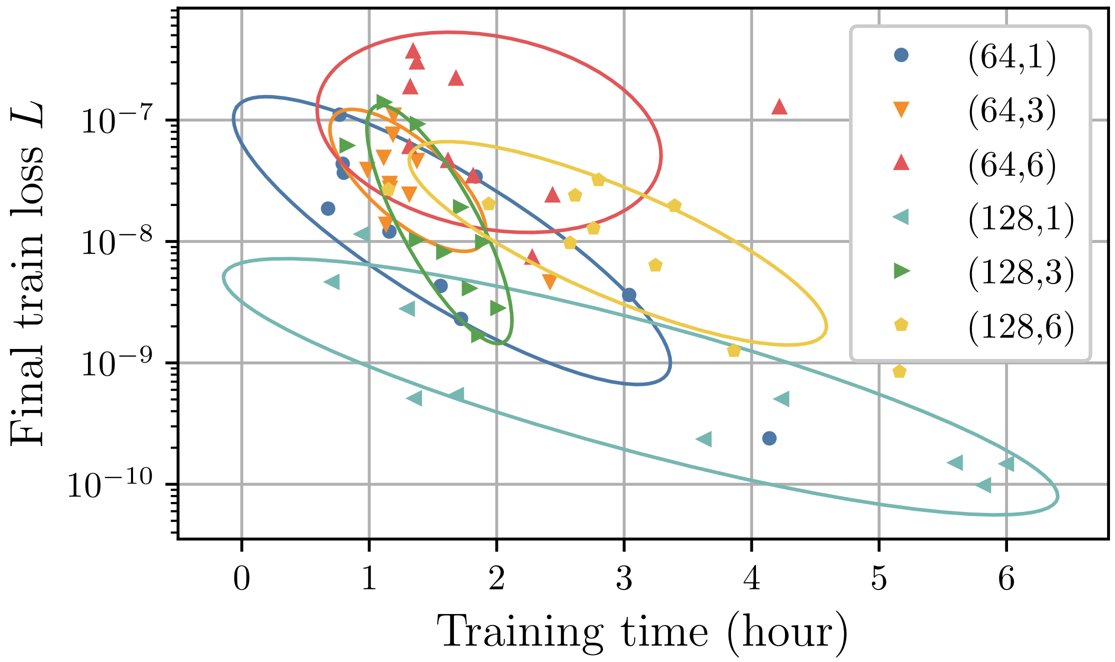


**Fig. 1.** (Color online) Dependency of final training loss and training time on network architecture. Marker shapes encode the architectural settings (layer width, number of skip-connected layers). For each configuration, individual points correspond to runs with distinct random initializations. The ellipses represent covariance ellipses for the respective clusters of samples.

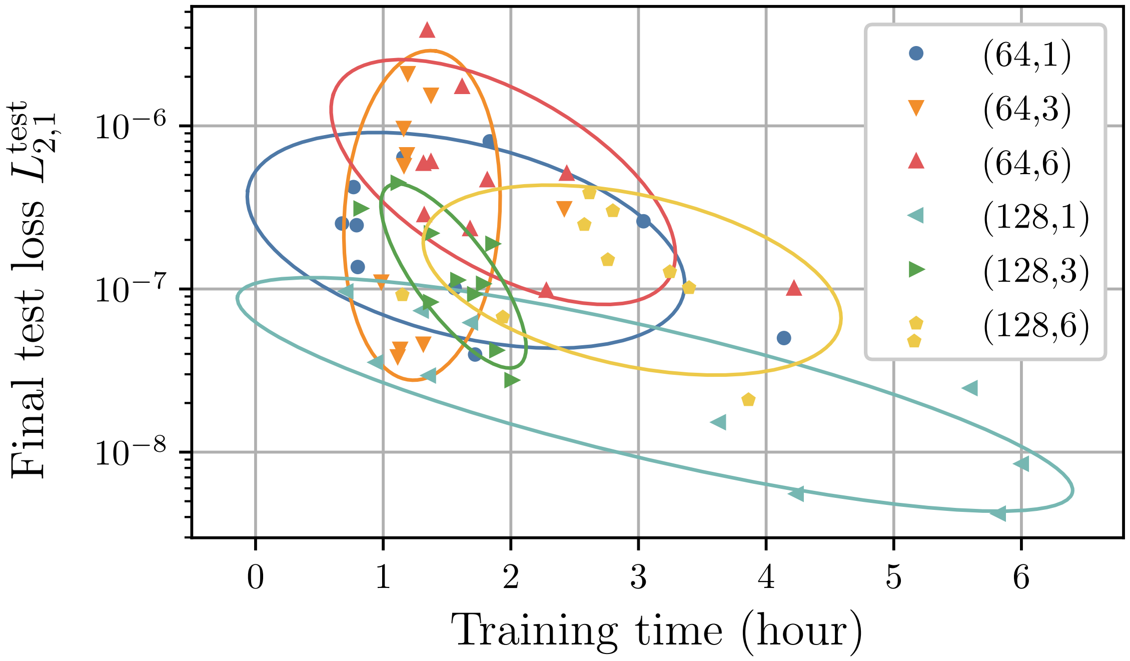


**Fig. 2.** (Color online) Dependency of final test loss $L_{2,1}^{\text{test}}$ and training time on network architecture. Marker shapes and covariance ellipses follow the same convention as in Fig 1.

**Table I.** The number of trainable parameters in each network architecture.The parameter set $(128, 1)$ corresponds to the architecture used in the main text.

| Layer width | # of skip-connected layers | # of params. in $\mathrm{NN}_p$ | # of params. in $\mathrm{NN}_\alpha$ | $N$ |
|---|---|---|---|---|
| 64 | 1 | 8,610 | 8,578 | 17,188 |
| 64 | 3 | 17,058 | 17,026 | 34,084 |
| 64 | 6 | 29,730 | 29,698 | 59,428 |
| 128 | 1 | 33,602 | 33,538 | 67,140 |
| 128 | 3 | 66,882 | 66,818 | 133,700 |
| 128 | 6 | 116,802 | 116,738 | 233,540 |

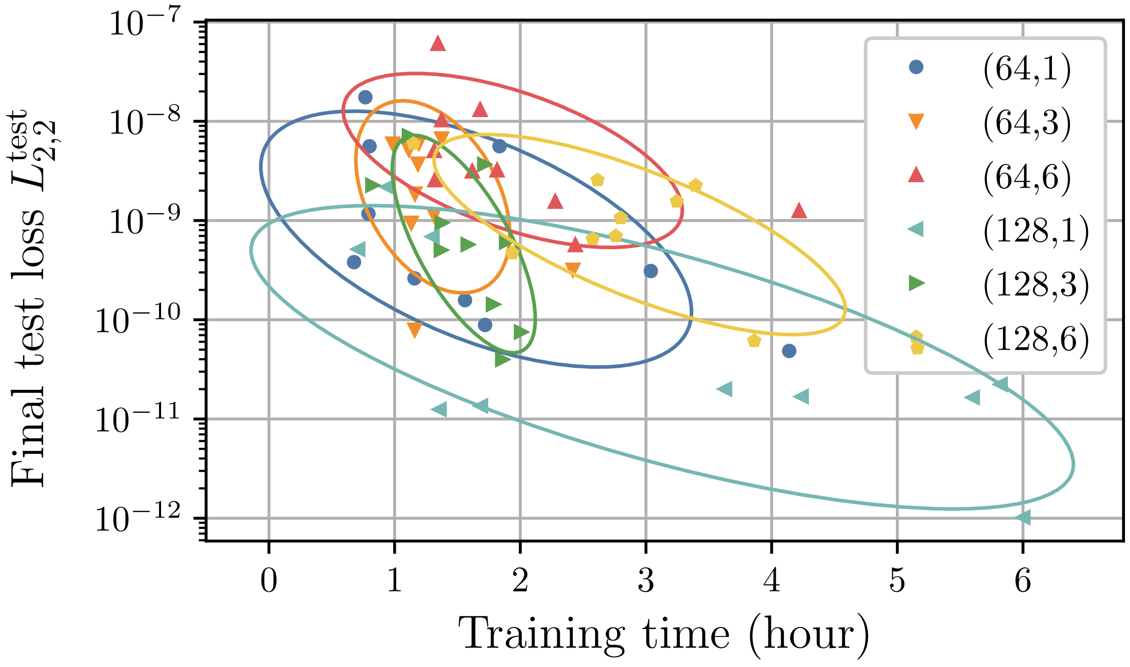


**Fig. 3.** (Color online) Dependency of final test loss $L^{\mathrm{test}}_{2,2}$ and training time on network architecture. Marker shapes and covariance ellipses follow the same convention as in Fig 1.

**References**


1) A. Jnini and F. Vella, arXiv:2505.21404. 10.48550/arXiv.2505.21404
